# Supplementary material for: Stochastic Model of Qudit Measurement for Superconducting Quantum Information Processing
Source: arXiv:2312.03754 source file (2024-04-15)
Supplement: Supplementary file 1 [file appendix_Master_Eqn.tex]

\chapter{Microscopic Derivation of the Master Equation}
\section{Microscopic Derivation of the Born-Markov Master Equation}
\section{The Redfield Master Equation}
\section{The Lindbald Master Equation}
    \begin{equation}
        \hat{H}_{\text{int}} 
        = \sum_{\alpha}
            \hat{S}_{\alpha} \otimes \hat{E}_{\alpha}
        \ \ \ \
        \hat{S}_{\alpha}^{\dagger} 
        = \hat{S}_{\alpha} 
        \ \ \ \ 
        \hat{E}_{\alpha}^{\dagger} 
        = \hat{E}_{\alpha} 
    \end{equation}
    \begin{equation}
        \hat{\Pi}(\Bar{\omega})
        = \sum_{\{a|\omega_a = \Bar{\omega}\}} \ket{a}\!\bra{a}
    \end{equation}
    \begin{equation}
        \hat{\Pi}(\Bar{\omega})
        = \hat{\Pi}(\Bar{\omega}) \hat{\Pi}(\Bar{\omega})
        \ \ \ \ 
        \hat{\Pi}^{\dagger}(\Bar{\omega}) = \hat{\Pi}(\Bar{\omega})
    \end{equation}
    \begin{equation}
        \hat{S}_{\alpha} (\omega) 
        = \sum_{\Bar{\omega}} \hat{\Pi}(\Bar{\omega} - \omega) \hat{S}_{\alpha} \hat{\Pi}(\Bar{\omega}) 
    \end{equation} 
    \begin{equation}
        \hat{S}_{\alpha}^{\dagger} (\omega) 
        = \sum_{\Bar{\omega}} \hat{\Pi}(\Bar{\omega}) \hat{S}_{\alpha} \hat{\Pi}(\Bar{\omega} - \omega)
    \end{equation} 
    \begin{equation}
        \sum_{\omega} \hat{S}_{\alpha} (\omega) 
        = \sum_{\omega} 
            \sum_{\Bar{\omega}} 
                \hat{\Pi}(\Bar{\omega} - \omega) 
                \hat{S}_{\alpha} 
                \hat{\Pi}(\Bar{\omega}) 
        = \sum_{\Bar{\omega}} 
                \hat{1}
                \hat{S}_{\alpha} 
                \hat{\Pi}(\Bar{\omega}) 
        = \hat{S}_{\alpha} \hat{1} = \hat{S}_{\alpha}
    \end{equation}
    \begin{equation} 
        \hat{S}_{\alpha} 
        = \sum_{\omega} \hat{S}_{\alpha} (\omega) 
        \ \ \ \ 
        \hat{S}_{\alpha} 
        = \sum_{\omega}
            \hat{S}_{\alpha}^{\dagger} (\omega) 
    \end{equation}

    \begin{align} 
        \hat{S}_{\alpha} 
        &= \sum_{\omega'} \hat{S}_{\alpha}^{\dagger} (\omega') 
    \nonumber \\
        \hat{S}_{\beta} 
        &= \sum_{\omega}
            \hat{S}_{\beta} (\omega) 
    \end{align}
    
    \begin{align} 
        \hat{S}_{\alpha} 
        &= \sum_{\omega'} \hat{S}_{\alpha} (\omega') 
    \nonumber \\
        \hat{S}_{\beta} 
        &= \sum_{\omega}
            \hat{S}_{\beta}^{\dagger} (\omega) 
    \end{align}

    \begin{equation}
        \left[\hat{H}_{\mathcal{S}}, \hat{S}_{\alpha}(\omega)\right]
        = - \omega \hat{S}_{\alpha}(\omega)
   \ \ \ \ 
        \left[\hat{H}_{\mathcal{S}}, \hat{S}^{\dagger}_{\alpha}(\omega)\right]
        = \omega \hat{S}^{\dagger}_{\alpha}(\omega)
    \end{equation}
    \begin{align}
        \frac{d}{dt} \hat{\Tilde{\rho}}_{\mathcal{S}}(t)
        &= -\frac{1}{\hbar^2}
            \int_{0}^{\infty} d\tau
            \sum_{\omega, \omega'} 
            \sum_{\alpha,\beta}
            \bigg\{
                G_{\alpha \beta}(\tau)
                \Big[
                e^{\ci \omega' t} \hat{S}_{\alpha}^{\dagger} (\omega') 
                e^{-\ci \omega (t-\tau)} \hat{S}_{\beta} (\omega) 
                \hat{\Tilde{\rho}}_{\mathcal{S}}(t)
    \nonumber \\[-2mm]
            & \ \ \ \ \ \ \ \ \ \ \ \ \ \ \ \ \ \ \ 
            \ \ \ \ \ \ \ \ \ \ \ \ \ \ \ \ \ \ \ 
            \ \ \ \ \ \ \ \ \ \ \ \ \ \ \ \ \ \ \ \ \ \ \ \ 
                - e^{-\ci \omega (t-\tau)} \hat{S}_{\beta} (\omega) 
                \hat{\Tilde{\rho}}_{\mathcal{S}}(t)
                e^{\ci \omega' t} \hat{S}_{\alpha}^{\dagger} (\omega') 
                \Big]
    \nonumber \\[-2mm]
            & \ \ \ \ \ \ \ \ \ \ \ 
            \ \ \ \ \ \ \ \ \ \ \ \ \ \ \ \ \ \ \ 
            + G_{\beta\alpha}(-\tau)
                \Big[
                \hat{\Tilde{\rho}}_{\mathcal{S}}(t)
                e^{\ci \omega (t-\tau)} \hat{S}_{\beta}^{\dagger}(\omega) 
                e^{-\ci \omega t} \hat{S}_{\alpha} (\omega') 
    \nonumber \\[-2mm]
            & \ \ \ \ \ \ \ \ \ \ \ \ \ \ \ \ \ \ \ 
            \ \ \ \ \ \ \ \ \ \ \ \ \ \ \ \ \ \ \ 
            \ \ \ \ \ \ \ \ \ \ \ \ \ \ \ \ \ \ \ \ \ \ \ \ 
            - e^{-\ci \omega t} \hat{S}_{\alpha} (\omega')  \hat{\Tilde{\rho}}_{\mathcal{S}}(t)
                e^{\ci \omega (t-\tau)} \hat{S}_{\beta}^{\dagger}(\omega) 
                \Big]
            \bigg\}
    \nonumber \\
        &= -\frac{1}{\hbar^2}
            \int_{0}^{\infty} d\tau
            \sum_{\omega, \omega'} 
            \sum_{\alpha,\beta}
            \bigg\{
                G_{\alpha \beta}(\tau) e^{\ci \omega \tau}
                e^{\ci (\omega' - \omega)t }
                \Big[
                \hat{S}_{\alpha}^{\dagger} (\omega') \hat{S}_{\beta} (\omega) \hat{\Tilde{\rho}}_{\mathcal{S}}(t)
                -  \hat{S}_{\beta} (\omega) \hat{\Tilde{\rho}}_{\mathcal{S}}(t) \hat{S}_{\alpha}^{\dagger} (\omega') 
                \Big]
    \nonumber \\[-2mm]
            & \ \ \ \ \ \ \ \ \ \ \ 
            \ \ \ \ \ \ \ \ \ \ \ \ \ \ \ \ \ \ \ 
            + G_{\beta\alpha}(-\tau) e^{-\ci \omega \tau}
            e^{-\ci (\omega' - \omega)t }
                \left[
                \hat{\Tilde{\rho}}_{\mathcal{S}}(t) \hat{S}_{\beta}^{\dagger}(\omega) \hat{S}_{\alpha} (\omega') 
                - \hat{S}_{\alpha} (\omega')  \hat{\Tilde{\rho}}_{\mathcal{S}}(t) \hat{S}_{\beta}^{\dagger}(\omega) 
                \right]
            \bigg\}
    \end{align}
    \begin{equation}
        \Gamma_{\alpha \beta} (\omega)
        = \int_0^{\infty} d\tau G_{\alpha \beta} (\tau) e^{\ci \omega \tau}
    \end{equation}
    \begin{equation}
        \Gamma_{\alpha \beta}^{*} (\omega)
        = \int_0^{\infty} d\tau G_{\alpha \beta}^* (\tau) e^{-\ci \omega \tau}
        = \int_0^{\infty} d\tau G_{\beta \alpha } (-\tau) e^{-\ci \omega \tau}
    \end{equation}
    
    \begin{align}
        \frac{d}{dt} \hat{\Tilde{\rho}}_{\mathcal{S}}(t)
    &= -\frac{1}{\hbar^2}
            \int_{0}^{\infty} d\tau
            \sum_{\omega} 
            \sum_{\alpha,\beta}
            \bigg\{
                \Gamma_{\alpha \beta}(\omega)
                \left[
                \hat{S}_{\alpha}^{\dagger} (\omega) \hat{S}_{\beta} (\omega) \hat{\Tilde{\rho}}_{\mathcal{S}}(t)
                -  \hat{S}_{\beta} (\omega) \hat{\Tilde{\rho}}_{\mathcal{S}}(t) \hat{S}_{\alpha}^{\dagger} (\omega) 
                \right]
            + \text{c.c.}
            \bigg\}
    \end{align}
    \begin{equation}
        \Gamma_{\alpha \beta} (\omega)
        = \frac{1}{2} \gamma_{\alpha \beta}(\omega)
            + \ci \Delta_{\alpha \beta}(\omega)
    \end{equation}
    \begin{equation}
        \gamma_{\alpha \beta}(\omega)
        = \Gamma_{\alpha \beta} (\omega) + \Gamma^*_{\beta \alpha } (\omega)
        = \int_{-\infty}^{\infty} d\tau     G_{\alpha \beta}(\tau) e^{\ci \omega \tau}
    \end{equation}
    \begin{equation}
        \Delta_{\alpha \beta}(\omega) 
        = \frac{1}{2\ci}
            \big[
                \Gamma_{\alpha \beta} (\omega) 
                - \Gamma^*_{\beta \alpha } (\omega)
            \big]
    \end{equation}
    \begin{align}
        \frac{d}{dt} \hat{\Tilde{\rho}}_{\mathcal{S}}(t)
        &= - \frac{\ci}{\hbar}
            \sum_{\omega} 
            \sum_{\alpha,\beta}
            \left[
            \frac{1}{\hbar} \Delta_{\alpha \beta}(\omega) \hat{S}^{\dagger}_{\alpha}(\omega) \hat{S}_{\beta}(\omega),
            \hat{\Tilde{\rho}}_{\mathcal{S}}(t)
            \right]
    \nonumber \\
        &\ \ \ \ \ \ \ \ \ \ \ \ \ \ \ \  + \sum_{\omega} \sum_{\alpha,\beta}
            \gamma_{\alpha \beta}(\omega)
            \frac{1}{\hbar^2}
            \left[
                \hat{S}_{\beta}(\omega)\hat{\Tilde{\rho}}_{\mathcal{S}}(t)
                \hat{S}^{\dagger}_{\alpha}(\omega)
                - \frac{1}{2} 
                \left\{
                    \hat{S}^{\dagger}_{\alpha}(\omega) \hat{S}_{\beta}(\omega),
                    \hat{\Tilde{\rho}}_{\mathcal{S}}(t)
                \right\}
            \right]
    \nonumber \\
        &= - \frac{\ci}{\hbar} 
            \left[
                \hat{H}_{\Delta},
                \hat{\Tilde{\rho}}_{\mathcal{S}}(t)
            \right]
            + \boldsymbol{\hat{\mathcal{D}}}
                \Bigsl[ 
                    \hat{\Tilde{\rho}}_{\mathcal{S}}(t)
                \Bigsr]
    \end{align}
    \begin{equation}
        \frac{d}{dt} \hat{\rho}_{\mathcal{S}}(t)
        = - \frac{\ci}{\hbar} 
            \left[
            \hat{H}_{\mathcal{S}} + \hat{H}_{\Delta},
            \hat{\rho}_{\mathcal{S}}(t)
            \right]
            + \boldsymbol{\hat{\mathcal{D}}}    
                \Bigsl[
                    \hat{\rho}_{\mathcal{S}}(t)
                \Bigsr]
    \end{equation}
    \begin{equation}
        \frac{d}{dt} \hat{\rho}_{\mathcal{S}}(t)
        = - \frac{\ci}{\hbar} 
            \left[
            \hat{H}_{\text{eff}},
            \hat{\rho}_{\mathcal{S}}(t)
            \right]
            + \sum_{\mu=1}^{N^2-1} k_{\mu} \!
                \left[
                \hat{L}_{\mu} \hat{\rho}_{\mathcal{S}}
                \hat{L}^{\dagger}_{\mu}
                - \frac{1}{2} 
                \left\{
                    \hat{L}_{\mu}^{\dagger} \hat{L}_{\mu},
                    \hat{\rho}_{\mathcal{S}}(t)
                \right\}
            \right]
    \end{equation}
