# Supplementary material for: Stochastic Model of Qudit Measurement for Superconducting Quantum Information Processing
Source: arXiv:2312.03754 source file (2024-04-15)
Supplement: Supplementary file 2 [file appendix_Quasiprob.tex]

% \chapter{Basics of Classical Stochastic Differential Equation and It\^{o} Calculus}
\chapter{Quasi-probabilities}

\section{Two-Dimensional Fourier Transform in the Phase Space}
\begin{equation}
    \alpha = X + \ci P
    \ \ \text{ and } \ \ 
    \lambda = X' + \ci P'
\end{equation}

% \begin{equation}
%     \lambda \alpha^* - \lambda^* \alpha
%     = 2 \ci (P' X - X'P)
% \end{equation}

\begin{equation}
    \alpha \lambda^* - \alpha^* \lambda
    = 2 \ci (P X' - X P')
\end{equation}

\begin{align}
    F(\alpha) 
    &= \int 
        \mathrm{d}^2 \lambda 
        e^{\alpha \lambda^* - \alpha^* \lambda}
        f(\lambda) 
\nonumber \\
    &= \iint 
        \mathrm{d}X'
        \mathrm{d}P'
        e^{2 \ci (P X' - X P')}
        f(X' + \ci P')
\nonumber \\
    &= \int 
        \mathrm{d}X'
        e^{2\ci P X'}
        \int 
            \mathrm{d}P'
            e^{- 2 \ci X P'}
            f(X' + \ci P')
\end{align}

\begin{equation}
    \alpha \hat{a}^{\dagger} - \alpha^* \hat{a}
    = 2 \ci (P \hat{X} - X\hat{P})
\end{equation}

\begin{equation}
    \hat{D}(\alpha) = e^{2 \ci (P \hat{X} - X\hat{P})}
\end{equation}

\section{Wigner Distribution}
\begin{equation}
    W(x,p) 
    = \frac{1}{\pi \hbar}
        \int_{-\infty}^{\infty}
            \mathrm{d} y
            e^{2\ci y p / \hbar}
            \bra{x-y} \hat{\rho} \ket{x+y}
\end{equation}
$\hbar = 1/2$
\begin{equation}
    W(X,P) 
    = \frac{2}{\pi}
        \int_{-\infty}^{\infty}
            \mathrm{d} Y
            e^{4\ci Y P}
            \bra{X-Y} \hat{\rho} \ket{X+Y}
\end{equation}
$\hbar = 1$
\begin{equation}
    W(X,P) 
    = \frac{1}{\pi}
        \int_{-\infty}^{\infty}
            \mathrm{d} Y
            e^{2\ci Y P}
            \bra{X-Y} \hat{\rho} \ket{X+Y}
\end{equation}

$x'=2y$
\begin{equation}
    W(X,P) 
    = \frac{1}{2 \pi \hbar}
        \int_{-\infty}^{\infty}
            \mathrm{d} x'
            e^{\ci x' p / \hbar}
            \bra{x-\frac{x'}{2}} \hat{\rho} \ket{x+\frac{x'}{2}}
\end{equation}

\section{Characteristic function}
\begin{equation}
    \chi_W (\alpha, \beta)
    = \Tr(\hat{\rho} e^{\alpha \hat{a}^{\dagger} - \beta \hat{a}})
\end{equation}
\begin{equation}
    \chi_W (\alpha, \alpha^*) = \chi_W(X,P)
    = \Tr[\hat{\rho} \hat{D}(\alpha)]
\end{equation}
\begin{equation}
    W(\alpha, \alpha^*)
    = \frac{1}{\pi^2} \int \mathrm{d}^2 \lambda \chi_W(\lambda,\lambda^*) e^{\alpha \lambda^* - \alpha^* \lambda}
\end{equation}
\begin{equation}
    \chi_{W}(\lambda)
    = \int \mathrm{d}^2 \alpha 
        W(\alpha) e^{-(\alpha \lambda^* - \alpha^* \lambda)}
\end{equation}
