# Supplementary material for: Stochastic Model of Qudit Measurement for Superconducting Quantum Information Processing
Source: arXiv:2312.03754 source file (2024-04-15)
Supplement: Supplementary file 3 [file appendix_Qudit_ME.tex]

\chapter{Measurement-Induced Dephasing}

\section{Master Equation for the Composite System (Qubit $+$ Resonator)}
\cite{PhysRevA.74.042318}
\begin{align}
    \dot{\hat{\rho}}_{\mathcal{SR}}(t)
    &= - \frac{\ci}{\hbar}
            \left[ 
                \hat{H}_{\mathcal{SR}}(t), 
                \hat{\rho}_{\mathcal{SR}}(t)
            \right]
        + \kappa 
            \mathcalboondox{D}[\hat{a}] 
            \hat{\rho}_{\mathcal{SR}}(t)
        + \gamma_1 
            \mathcalboondox{D}[\hat{\sigma}] 
            \hat{\rho}_{\mathcal{SR}}(t)
        + \frac{\gamma_{\phi}}{2} 
            \mathcalboondox{D}[\hat{\sigma}_{z}]
            \hat{\rho}_{\mathcal{SR}}(t)
\nonumber \\
    &\approx - \frac{\ci}{\hbar}
            \left[ 
                \hat{H}_{\mathcal{SR}}(t), 
                \hat{\rho}_{\mathcal{SR}}(t)
            \right]
        + \kappa 
            \mathcalboondox{D}[\hat{a}] 
            \hat{\rho}_{\mathcal{SR}}(t)
        + \frac{\gamma_2}{2} 
            \mathcalboondox{D}[\hat{\sigma}_{z}]
            \hat{\rho}_{\mathcal{SR}}(t)
\end{align}
where $\gamma_2 = \gamma_{\phi} + \gamma_1/2$

\begin{equation}
    \mathcalboondox{D}[\hat{L}] \hat{\rho}
    = \hat{L} \hat{\rho} \hat{L}^{\dagger}
        - \frac{1}{2} \left\{\hat{\rho},  \hat{L}^{\dagger} \hat{L} \right\}
\end{equation}

\begin{equation}
    \hat{H}_{\mathcal{SR}}(t)
    \approx - \frac{1}{2} \hbar \omega_{\text{q}} \hat{\sigma}_z
        + \hbar \omega_r \hat{a}^{\dagger} \hat{a} 
        - \hbar \chi \hat{\sigma}_z \hat{a}^{\dagger} \hat{a}
        + \hbar \epsilon(t) \!  \left( \hat{a} e^{\ci \omega t} + \hat{a}^{\dagger} e^{-\ci \omega t}\right)
\end{equation}

\begin{equation}
    \hat{H}_{\mathcal{SR}}^{\mathrm{d}}
    \approx - \frac{1}{2} \hbar \omega_{\text{q}} \hat{\sigma}_z
        + \hbar \Delta_{\text{rd}} \hat{a}^{\dagger} \hat{a} 
        - \hbar \chi \hat{\sigma}_z \hat{a}^{\dagger} \hat{a}
        + \hbar \epsilon(t) \! 
            \left( 
                \hat{a} 
                + \hat{a}^{\dagger} 
            \right)
\end{equation}

If we define 
\begin{equation}
    \hat{\rho}_{ab}(t) = \bra{a}\hat{\rho}_{\mathcal{SR}}(t)\ket{b}
\end{equation}

\begin{equation}
    \hat{\rho}_{\mathcal{SR}}(t)
    = \sum_{a,b \in \{e,g\}}
        \hat{\rho}_{ab}(t)
        \ket{a} \! \bra{b} 
    = \hat{\rho}_{gg}
        \ket{g} \! \bra{g} 
        + \hat{\rho}_{ge}
        \ket{g} \! \bra{e} 
        + \hat{\rho}_{eg}
        \ket{e} \! \bra{g} 
        + \hat{\rho}_{ee}
        \ket{e} \! \bra{e} 
\end{equation}

\begin{align}
    \bra{g}\hat{H}_{\mathcal{SR}}^{\mathrm{d}}\ket{g}
    &= - \frac{1}{2} \hbar \omega_{\text{q}} 
        - \hbar (\chi - \Delta_{\text{rd}}) \hat{a}^{\dagger}\hat{a}
        + \hbar \epsilon(t) \!  \left( \hat{a} + \hat{a}^{\dagger} \right)
\\
    \bra{e}\hat{H}_{\mathcal{SR}}^{\mathrm{d}}\ket{e}
    &= \frac{1}{2} \hbar \omega_{\text{q}} 
        + \hbar (\chi + \Delta_{\text{rd}}) \hat{a}^{\dagger}\hat{a}
        + \hbar \epsilon(t) \!  \left( \hat{a} + \hat{a}^{\dagger}\right)
\\
    \bra{g}\hat{H}_{\mathcal{SR}}^{\mathrm{d}}\ket{e} 
    &= \bra{e}\hat{H}_{\mathcal{SR}}^{\mathrm{d}}\ket{g} 
    = \hat{0}
\end{align}

\begin{equation}
    \bra{a}
        \left[ 
            \hat{H}_{\mathcal{SR}}^{\mathrm{d}}, 
            \hat{\rho}_{\mathcal{SR}}
        \right]
        \ket{b} 
    = \bra{a}
            \hat{H}_{\mathcal{SR}}^{\mathrm{d}}
            \ket{a} 
            \hat{\rho}_{ab}
        - \hat{\rho}_{ab}
            \bra{b}
            \hat{H}_{\mathcal{SR}}^{\mathrm{d}}
            \ket{b} 
\end{equation}

\begin{align}
    \bra{g}\left[ 
                \hat{H}_{\mathcal{SR}}^{\mathrm{d}}, 
                \hat{\rho}_{\mathcal{SR}}
            \right]\ket{g} 
    &= - \hbar (\chi - \Delta_{\text{rd}}) 
        \left[ 
            \hat{a}^{\dagger}\hat{a}, \hat{\rho}_{gg}
        \right]
        + \hbar \epsilon(t) \!  
            \left[ 
                \hat{a} + \hat{a}^{\dagger},
                \hat{\rho}_{gg} 
            \right]
\\
    \bra{e}\left[ 
                \hat{H}_{\mathcal{SR}}^{\mathrm{d}}, 
                \hat{\rho}_{\mathcal{SR}}
            \right]\ket{e} 
    &= \hbar (\chi + \Delta_{\text{rd}}) 
        \left[ 
            \hat{a}^{\dagger}\hat{a}, \hat{\rho}_{gg}
        \right]
        + \hbar \epsilon(t) \!  
            \left[ 
                \hat{a} + \hat{a}^{\dagger},
                \hat{\rho}_{gg} 
            \right]
\\
    \bra{g}\left[ 
                \hat{H}_{\mathcal{SR}}^{\mathrm{d}}, 
                \hat{\rho}_{\mathcal{SR}}
            \right]\ket{e} 
    &= - \hbar \omega_{\text{q}} \hat{\rho}_{ge}
        + \hbar \Delta_{\text{rd}}
        \left[ 
            \hat{a}^{\dagger}\hat{a}, \hat{\rho}_{ge}
        \right]
        - \hbar \chi \left\{
            \hat{a}^{\dagger}\hat{a}, \hat{\rho}_{ge}
        \right\}
        + \hbar \epsilon(t) \!  
            \left[ 
                \hat{a} + \hat{a}^{\dagger},
                \hat{\rho}_{ge} 
            \right]
\\
    \bra{e}\left[ 
                \hat{H}_{\mathcal{SR}}^{\mathrm{d}}, 
                \hat{\rho}_{\mathcal{SR}}
            \right]\ket{g} 
    &= \hbar \omega_{\text{q}} \hat{\rho}_{eg}
        + \hbar \Delta_{\text{rd}}
        \left[ 
            \hat{a}^{\dagger}\hat{a}, \hat{\rho}_{eg}
        \right]
        + \hbar \chi \left\{
            \hat{a}^{\dagger}\hat{a}, \hat{\rho}_{eg}
        \right\}
        + \hbar \epsilon(t) \!  
            \left[ 
                \hat{a} + \hat{a}^{\dagger},
                \hat{\rho}_{eg} 
            \right]
\end{align}

\begin{align}
    \bra{a}
        \mathcalboondox{D}[\hat{\sigma}_{z}]
        \hat{\rho}_{\mathcal{SR}}
    \ket{b} 
    &= \bra{a} 
        \hat{\sigma}_z 
        \hat{\rho}_{\mathcal{SR}}     
        \hat{\sigma}_z 
        \ket{b}
        - \frac{1}{2} 
            \bra{a} 
            \left \{
                \hat{1}, 
                \hat{\rho}_{\mathcal{SR}} 
            \right \} 
            \ket{b}
\nonumber \\
    &= (-1)^{a+b}
        \hat{\rho}_{ab} - \hat{\rho}_{ab}
    = \begin{cases}
        \hat{0}, & \text{ if } a = b, \\
        - 2\hat{\rho}_{ab}, & \text{ if } a \neq b.
        \end{cases}
\end{align}

\begin{align}
    \dot{\hat{\rho}}_{gg}
    &= \ci (\chi - \Delta_{\text{rd}}) \left[ 
            \hat{a}^{\dagger}\hat{a}, \hat{\rho}_{gg}
        \right]
        - \ci \epsilon(t) \!  
            \left[ 
                \hat{a} + \hat{a}^{\dagger},
                \hat{\rho}_{gg} 
            \right]
            + \kappa \mathcalboondox{D}[\hat{a}]
                \hat{\rho}_{gg}
\\
    \dot{\hat{\rho}}_{ee}
    &= - \ci (\chi + \Delta_{\text{rd}}) \left[ 
            \hat{a}^{\dagger}\hat{a}, \hat{\rho}_{ee}
        \right]
        - \ci \epsilon(t) \!  
            \left[ 
                \hat{a} + \hat{a}^{\dagger},
                \hat{\rho}_{ee} 
            \right]
            + \kappa \mathcalboondox{D}[\hat{a}]
                \hat{\rho}_{ee}
\\
    \dot{\hat{\rho}}_{ge}
    &= \ci \omega_{\text{q}} \hat{\rho}_{ge} 
        - \ci \Delta_{\text{rd}} \left[ 
            \hat{a}^{\dagger}\hat{a}, \hat{\rho}_{ge}
        \right] \!
        + \ci\chi \left\{
            \hat{a}^{\dagger}\hat{a}, \hat{\rho}_{ge}
        \right\}
        - \ci \epsilon(t) \!  
            \left[ 
                \hat{a} + \hat{a}^{\dagger},
                \hat{\rho}_{ge} 
            \right] \!
        + \kappa \mathcalboondox{D}[\hat{a}]
                \hat{\rho}_{ge}
        - \gamma_2 \hat{\rho}_{ge}
\\
    \dot{\hat{\rho}}_{eg}
    &= - \ci \omega_{\text{q}} \hat{\rho}_{eg} 
        - \ci \Delta_{\text{rd}} \left[ 
            \hat{a}^{\dagger}\hat{a}, \hat{\rho}_{eg}
        \right] \!
        - \ci\chi \left\{
            \hat{a}^{\dagger}\hat{a}, \hat{\rho}_{eg}
        \right\}
        - \ci \epsilon(t) \!  
            \left[ 
                \hat{a} + \hat{a}^{\dagger},
                \hat{\rho}_{eg} 
            \right] \!
        + \kappa \mathcalboondox{D}[\hat{a}]
                \hat{\rho}_{eg}
        - \gamma_2 \hat{\rho}_{eg}
\end{align}

\begin{equation}
    \hat{\rho}_{ab} 
    = \int \mathrm{d}^2 \alpha
        \int \mathrm{d}^2 \beta
            \frac{\ket{\alpha}\!\bra{\beta^*}}{\braket{\beta^*}{\alpha}} P_{ab}(\alpha, \beta)
\end{equation}

\section{Master Equation for the Composite System (Qutrit $+$ Resonator)}

\begin{align}
    \dot{\hat{\rho}}_{\mathcal{SR}}(t)
    &= - \frac{\ci}{\hbar}
            \left[ 
                \hat{H}_{\mathcal{SR}}(t), 
                \hat{\rho}_{\mathcal{SR}}(t)
            \right]
        + \kappa 
            \mathcalboondox{D}[\hat{a}] 
            \hat{\rho}_{\mathcal{SR}}(t)
        + \frac{\gamma_{2,ge}}{2} 
            \mathcalboondox{D}\big[\ket{g}\!\bra{g} - \ket{e}\!\bra{e}\big]
            \hat{\rho}_{\mathcal{SR}}(t)
\nonumber \\ \label{eq:general_qutrit_cavity_master_equation}
        & \ \ \ \ \ \ \ \ \ \ \ \ \ \ \  
        + \frac{\gamma_{2,gf}}{2} 
            \mathcalboondox{D}\big[\ket{g}\!\bra{g} - \ket{f}\!\bra{f}\big]
            \hat{\rho}_{\mathcal{SR}}(t)
        + \frac{\gamma_{2,ef}}{2} 
            \mathcalboondox{D}\big[\ket{e}\!\bra{e} - \ket{f}\!\bra{f}\big]
            \hat{\rho}_{\mathcal{SR}}(t)
\end{align}

The qutrit + cavity Hamiltonian in the dispersive regime subject to a classical drive $\varepsilon_{\text{d}}(t)$ (under the RWA) is given by
\begin{align}
    \frac{\hat{H}^{\text{disp}}_{\mathcal{SR}}(t)}{\hbar}
    &= \omega_{\text{q}} \ket{e}\!\bra{e}
        + ( 2\omega_{\text{q}} + \alpha_{\text{q}} ) 
            \ket{f}\!\bra{f}
        + \omega_{\text{r}} \hat{a}^{\dagger} \hat{a} 
        + \chi_{\text{qr}} 
            (\ket{e}\!\bra{e} + 2 \ket{f}\!\bra{f})\hat{a}^{\dagger} \hat{a} 
        - \left[ 
            \varepsilon_{\text{d}}(t) \hat{a}^{\dagger}
            + \varepsilon_{\text{d}}^{*}(t) \hat{a} 
        \right]
\nonumber \\
    &= \omega_{\text{q}} \ket{e}\!\bra{e}
        + (2\omega_{\text{q}} + \alpha_{\text{q}}) \ket{f}\!\bra{f}
        + \omega_{\text{r}} \hat{a}^{\dagger} \hat{a} 
        + \chi_{\text{qr}} (\ket{e}\!\bra{e} + 2 \ket{f}\!\bra{f})\hat{a}^{\dagger} \hat{a} 
\nonumber \\
    & \ \ \ \ \ \ \ \ \ \ \ \ \ \ \ \ \ \ \ \ \ \ \ \ \ \ \ \ \ \ \ \ \ \ \ \ \ \ \ \ \ \ \ \ \ \ \ \ \ \ \ \ \ 
        - \left[
            \sqrt{\kappa} \bar{a}_{\text{in}} 
                e^{-\ci\omega_{\text{d}} t} 
                \,\hat{a}^{\dagger} 
            + \sqrt{\kappa} \bar{a}_{\text{in}}^{*} 
                e^{\ci\omega_{\text{d}} t} 
                \, \hat{a} 
        \right]
\end{align}
The subsequent calculation can be simplified if we move the cavity part of the Hamiltonian to a rotating frame with the frequency $\omega_{\text{d}}$. Then the time-varying drive $\varepsilon_{\text{d}}(t)$ reduces to a complex scalar $\epsilon = \sqrt{\kappa} \bar{a}_{\text{in}}$ and the Hamiltonian is now time-independent
\begin{equation}
    \frac{\hat{H}_{\mathcal{SR},\text{rot}}^{\mathrm{disp}}}{\hbar}
    = \omega_{\text{q}} \ket{e}\!\bra{e}
        + (2\omega_{\text{q}} + \alpha_{\text{q}}) \ket{f}\!\bra{f}
        + \Delta_{\text{rd}} \hat{a}^{\dagger} \hat{a} 
        + \chi_{\text{qr}} (\ket{e}\!\bra{e} + 2 \ket{f}\!\bra{f})\hat{a}^{\dagger} \hat{a} 
        - \left( 
            \epsilon \hat{a}^{\dagger}
            + \epsilon^* \hat{a}
        \right).
\end{equation}
Thus, the qutrit + cavity master equation in the rotating frame is obtained by using $\hat{H}_{\mathcal{SR},\text{rot}}^{\mathrm{disp}}$ as $\hat{H}_{\mathcal{SR}}$ in Eq.(\ref{eq:general_qutrit_cavity_master_equation}). 

To solve the master equation, we define 
\begin{equation}
    \hat{\rho}_{ab}(t) = \bra{a}\hat{\rho}_{\mathcal{SR}}(t)\ket{b}
    \in L(\mathscr{H}_{\mathcal{R}})
\end{equation}
for $a,b \in \{ g, e ,f\}$; in other words, the reduced density operator can be decomposed as
\begin{align}
    \hat{\rho}_{\mathcal{SR}}(t)
    &= \hat{\rho}_{gg}
        \ket{g} \! \bra{g} 
        + \hat{\rho}_{ge}
        \ket{g} \! \bra{e} 
        + \hat{\rho}_{gf}
        \ket{g} \! \bra{f} 
\nonumber \\
    & \ \ \ \ 
        + \hat{\rho}_{eg}
        \ket{e} \! \bra{g} 
        + \hat{\rho}_{ee}
        \ket{e} \! \bra{e} 
        + \hat{\rho}_{ef}
        \ket{e} \! \bra{f} 
\nonumber \\
    & \ \ \ \ 
        + \hat{\rho}_{fg}
        \ket{f} \! \bra{g} 
        + \hat{\rho}_{fe}
        \ket{f} \! \bra{e} 
        + \hat{\rho}_{ff}
        \ket{f} \! \bra{f},
\end{align}
and, after expanding the master equation using the nine operators, we obtain nine coupled operator differential equations
\begin{align} \label{eq:rho_qutrit_and_cavity_gg}
    \dot{\hat{\rho}}_{gg}
    &= - \ci \Delta_{\text{rd}} \left[ 
            \hat{a}^{\dagger}\hat{a}, \hat{\rho}_{gg}
        \right]
        + \ci 
            \left[ 
                \epsilon \hat{a}^{\dagger}
                    + \epsilon^* \hat{a},
                \hat{\rho}_{gg} 
            \right]
            + \kappa \mathcalboondox{D}[\hat{a}]
                \hat{\rho}_{gg}
\\ \label{eq:rho_qutrit_and_cavity_ee}
    \dot{\hat{\rho}}_{ee}
    &= - \ci (\chi_{\text{qr}} + \Delta_{\text{rd}}) \left[ 
            \hat{a}^{\dagger}\hat{a}, \hat{\rho}_{ee}
        \right]
        + \ci \left[ 
                \epsilon \hat{a}^{\dagger}
                    + \epsilon^* \hat{a},
                \hat{\rho}_{ee} 
            \right]
            + \kappa \mathcalboondox{D}[\hat{a}]
                \hat{\rho}_{ee}
\\ \label{eq:rho_qutrit_and_cavity_ff}
    \dot{\hat{\rho}}_{ff}
    &= - \ci (2\chi_{\text{qr}} + \Delta_{\text{rd}}) \left[ 
            \hat{a}^{\dagger}\hat{a}, \hat{\rho}_{ff}
        \right]
        + \ci \left[ 
                \epsilon \hat{a}^{\dagger}
                    + \epsilon^* \hat{a},
                \hat{\rho}_{ff} 
            \right]
            + \kappa \mathcalboondox{D}[\hat{a}]
                \hat{\rho}_{ff}
\\ \label{eq:rho_qutrit_and_cavity_ge}
    \dot{\hat{\rho}}_{ge}
    &= \ci \omega_{\text{q}} \hat{\rho}_{ge} 
        - \ci \Delta_{\text{rd}} \left[ 
            \hat{a}^{\dagger}\hat{a}, \hat{\rho}_{ge}
        \right] \!
        + \ci\chi_{\text{qr}} \hat{\rho}_{ge}
            \hat{a}^{\dagger}\hat{a}
\nonumber \\
    & \ \ \ \ \ \ \ \ \ \ \ \ \ \ \ \ \ \ \ \ \ \ \ \ 
        + \ci \left[ 
                \epsilon \hat{a}^{\dagger}
                    + \epsilon^* \hat{a},
                \hat{\rho}_{ge} 
            \right] \!
        + \kappa \mathcalboondox{D}[\hat{a}]
                \hat{\rho}_{ge}
        - \gamma_{2,ge} \hat{\rho}_{ge}
\\ \label{eq:rho_qutrit_and_cavity_eg}
    \dot{\hat{\rho}}_{eg}
    &= - \ci \omega_{\text{q}} \hat{\rho}_{eg} 
        + \ci \Delta_{\text{rd}} \left[ 
            \hat{a}^{\dagger}\hat{a}, \hat{\rho}_{eg}
        \right] \!
        - \ci\chi_{\text{qr}} \hat{\rho}_{eg}
            \hat{a}^{\dagger}\hat{a}
\nonumber \\
    & \ \ \ \ \ \ \ \ \ \ \ \ \ \ \ \ \ \ \ \ \ \ \ \ 
        - \ci \left[ 
                \epsilon \hat{a}^{\dagger}
                    + \epsilon^* \hat{a},
                \hat{\rho}_{eg} 
            \right] \!
        + \kappa \mathcalboondox{D}[\hat{a}]
                \hat{\rho}_{eg}
        - \gamma_{2,eg} \hat{\rho}_{eg}
\\ \label{eq:rho_qutrit_and_cavity_gf}
    \dot{\hat{\rho}}_{gf}
    &= \ci (2\omega_{\text{q}} + \alpha_{\text{q}})\hat{\rho}_{gf} 
        - \ci \Delta_{\text{rd}} \left[ 
            \hat{a}^{\dagger}\hat{a}, \hat{\rho}_{gf}
        \right] \!
        + \ci 2 \chi_{\text{qr}} \hat{\rho}_{gf}
            \hat{a}^{\dagger}\hat{a}
\nonumber \\
    & \ \ \ \ \ \ \ \ \ \ \ \ \ \ \ \ \ \ \ \ \ \ \ \ 
        + \ci \left[ 
                \epsilon \hat{a}^{\dagger}
                    + \epsilon^* \hat{a},
                \hat{\rho}_{gf} 
            \right] \!
        + \kappa \mathcalboondox{D}[\hat{a}]
                \hat{\rho}_{gf}
        - \gamma_{2,gf} \hat{\rho}_{gf}
\\ \label{eq:rho_qutrit_and_cavity_fg}
    \dot{\hat{\rho}}_{fg}
    &= -\ci (2\omega_{\text{q}} + \alpha_{\text{q}})\hat{\rho}_{fg} 
        + \ci \Delta_{\text{rd}} \left[ 
            \hat{a}^{\dagger}\hat{a}, \hat{\rho}_{fg}
        \right] \!
        - \ci 2 \chi_{\text{qr}} \hat{\rho}_{fg}
            \hat{a}^{\dagger}\hat{a}
\nonumber \\
    & \ \ \ \ \ \ \ \ \ \ \ \ \ \ \ \ \ \ \ \ \ \ \ \ 
        - \ci \left[ 
                \epsilon \hat{a}^{\dagger}
                    + \epsilon^* \hat{a},
                \hat{\rho}_{fg} 
            \right] \!
        + \kappa \mathcalboondox{D}[\hat{a}]
                \hat{\rho}_{fg}
        - \gamma_{2,fg} \hat{\rho}_{fg}
\\ \label{eq:rho_qutrit_and_cavity_ef}
    \dot{\hat{\rho}}_{ef}
    &= \ci (\omega_{\text{q}} + \alpha_{\text{q}}) \hat{\rho}_{ef} 
        - \ci \Delta_{\text{rd}} \left[ 
            \hat{a}^{\dagger}\hat{a}, \hat{\rho}_{ef}
        \right] \!
        + \ci \chi_{\text{qr}} (2\hat{\rho}_{ef}
            \hat{a}^{\dagger}\hat{a}
            - \hat{a}^{\dagger}\hat{a} \hat{\rho}_{ef})
\nonumber \\
    & \ \ \ \ \ \ \ \ \ \ \ \ \ \ \ \ \ \ \ \ \ \ \ \
        + \ci \left[ 
                \epsilon \hat{a}^{\dagger}
                    + \epsilon^* \hat{a},
                \hat{\rho}_{ef} 
            \right] \!
        + \kappa \mathcalboondox{D}[\hat{a}]
                \hat{\rho}_{ef}
        - \gamma_{2,ef} \hat{\rho}_{ef}
\\ \label{eq:rho_qutrit_and_cavity_fe}
    \dot{\hat{\rho}}_{fe}
    &= -\ci (\omega_{\text{q}} + \alpha_{\text{q}}) \hat{\rho}_{fe} 
        + \ci \Delta_{\text{rd}} \left[ 
            \hat{a}^{\dagger}\hat{a}, \hat{\rho}_{fe}
        \right] \!
        - \ci \chi_{\text{qr}} (2\hat{\rho}_{fe}
            \hat{a}^{\dagger}\hat{a}
            - \hat{a}^{\dagger}\hat{a} \hat{\rho}_{fe})
\nonumber \\
    & \ \ \ \ \ \ \ \ \ \ \ \ \ \ \ \ \ \ \ \ \ \ \ \
        - \ci \left[ 
                \epsilon \hat{a}^{\dagger}
                    + \epsilon^* \hat{a},
                \hat{\rho}_{fe} 
            \right] \!
        + \kappa \mathcalboondox{D}[\hat{a}]
                \hat{\rho}_{fe}
        - \gamma_{2,fe} \hat{\rho}_{fe}.
\end{align}

Note that each operator $\hat{\rho}_{ab}$ lives in an infinite dimensional space since $\mathscr{H}_{\mathcal{R}}$ is a Fock space. Nevertheless, it's possible to find a closed-form solution by invoking the complex $P$-representation
\begin{equation}
    \hat{\rho}_{ab}(t) 
    = \int \mathrm{d}^2 \alpha
        \int \mathrm{d}^2 \beta
            \frac{\ket{\alpha}\!\bra{\beta^*}}{\braket{\beta^*}{\alpha}} P_{ab}(\alpha, \beta, t).
\end{equation}
The reader can verify that the action of the creation and annihilation operators in the operator space can be translated to some simple operations in the complex $P$-representation:
\begin{align} \label{eq:operator_correspondance_1}
    \hat{a} \hat{\rho} (t)  
    &\ \ \longrightarrow \ \ 
    \alpha 
    P(\alpha, \beta, t)
\\ \label{eq:operator_correspondance_2}
    \hat{a}^{\dagger} \hat{\rho} (t)  
    &\ \ \longrightarrow \ \ 
    \left(
        \beta - \frac{\partial}{\partial \alpha} 
    \right)
    P(\alpha, \beta, t)
\\ \label{eq:operator_correspondance_3}
    \hat{\rho} (t) \hat{a}^{\dagger}
    &\ \ \longrightarrow \ \ 
    \beta P(\alpha, \beta, t)
\\ \label{eq:operator_correspondance_4}
    \hat{\rho} (t) \hat{a} 
    &\ \ \longrightarrow \ \ 
    \left(
        \alpha - \frac{\partial}{\partial \beta} 
    \right) P(\alpha, \beta, t)
\end{align}
As an example, let us use Eq.(\ref{eq:operator_correspondance_1}) to (\ref{eq:operator_correspondance_4}) to transform Eq.(\ref{eq:rho_qutrit_and_cavity_gg}) into a scalar equation:
\begin{align}
    \dot{P}_{gg}
    &= - \ci \Delta_{\text{rd}}
            \left [
                \left(
                    \beta - \frac{\partial}{\partial \alpha} 
                \right)
                (\alpha P_{gg})
                - \left(
                    \alpha - \frac{\partial}{\partial \beta} 
                \right)
                (\beta P_{gg})
            \right]
\nonumber \\
    & \ \ \ \ \ \ \ \ \ \ \ \ 
        + \ci 
            \left[
                \epsilon 
                    \left(
                        \beta 
                        - \frac{\partial}{\partial \alpha} 
                    \right) P_{gg}
                + \epsilon^* \alpha P_{gg}
                - \epsilon \beta P_{gg}
                - \epsilon^* 
                    \left(
                        \alpha 
                        - \frac{\partial}{\partial \beta} 
                    \right) P_{gg}
            \right]
\nonumber \\
    & \ \ \ \ \ \ \ \ \ \ \ \
        + \kappa 
            \left[
                \alpha \beta P_{gg}
                - \frac{1}{2} 
                \left(
                    \beta - \frac{\partial}{\partial \alpha} 
                \right)
                (\alpha P_{gg})
                - \frac{1}{2} \left(
                    \alpha - \frac{\partial}{\partial \beta} 
                \right)
                (\beta P_{gg})
            \right]
\nonumber \\
    &= \frac{\partial}{\partial \alpha}
        \left[
            \left(
                -\ci \epsilon 
                + \ci \Delta_{\text{rd}} \alpha 
                + \frac{\kappa \alpha}{2} 
            \right) 
            P_{gg}
        \right]
        + \frac{\partial}{\partial \beta}
        \left[
            \left(
                \ci \epsilon^{*} 
                - \ci \Delta_{\text{rd}} \beta
                + \frac{\kappa \beta}{2}
            \right) 
            P_{gg}
        \right],
\end{align}
where $\partial_t P_{gg} (\alpha, \beta, t)$ is shorthanded as $\dot{P}_{gg}$. By applying the same procedure to the other eight operators, we get, in total, nine coupled scalar differential equations
\begin{align} \label{eq:complex_P_gg}
    \dot{P}_{gg}
    &= \frac{\partial}{\partial \alpha}
        \left[
            (-\ci \epsilon 
            + \ci \Delta_{\text{rd}} \alpha 
            + \kappa \alpha/2) 
            P_{gg}
        \right]
        + \frac{\partial}{\partial \beta}
        \left[
            (\ci \epsilon^{*}  
            - \ci \Delta_{\text{rd}} \beta
            + \kappa \beta/2) 
            P_{gg}
        \right]
\\ \label{eq:complex_P_ee}
    \dot{P}_{ee}
    &= \frac{\partial}{\partial \alpha}
        \left[
            (-\ci \epsilon 
            + \ci \chi_{\text{qr}} \alpha 
            + \ci \Delta_{\text{rd}} \alpha 
            + \kappa \alpha/2) 
            P_{ee}
        \right]
        + \frac{\partial}{\partial \beta}
        \left[
            (\ci \epsilon^{*} 
            - \ci \chi_{\text{qr}} \beta
            - \ci \Delta_{\text{rd}} \beta
            + \kappa \beta/2) 
            P_{ee}
        \right]
\\ \label{eq:complex_P_ff}
    \dot{P}_{ff}
    &= \frac{\partial}{\partial \alpha}
        \left[
            (-\ci \epsilon 
            + \ci 2\chi_{\text{qr}} \alpha 
            + \ci \Delta_{\text{rd}} \alpha 
            + \kappa \alpha/2) 
            P_{ff}
        \right]
        + \frac{\partial}{\partial \beta}
        \left[
            (\ci \epsilon^{*} 
            - \ci 2\chi_{\text{qr}} \beta
            - \ci \Delta_{\text{rd}} \beta
            + \kappa \beta/2) 
            P_{ff}
        \right]
\\
    \dot{P}_{ge}
    &= \frac{\partial}{\partial \alpha}
        \left[
            (- \ci \epsilon 
            + \ci \Delta_{\text{rd}} \alpha 
            + \kappa \alpha/2) 
            P_{ge}
        \right]
        + \frac{\partial}{\partial \beta}
        \left[
            (\ci \epsilon^{*}  
            - \ci \chi_{\text{qr}} \beta
            - \ci \Delta_{\text{rd}} \beta
            + \kappa \beta/2) 
            P_{ge}
        \right]
\nonumber \\ \label{eq:complex_P_ge}
    & \ \ \ \ \ \ \ \ \ \ \ \ \ \ \ \ \ \ \ \ \ \ \ \ \ \ \ \ \ \ \ \ \ \ \ \ \ \ \ \ \ \ \ \ \ \ \ \ \ \ \ \ \ \ \ \ \ \ \ \
        + \ci \chi_{\text{qr}} \alpha \beta P_{ge}
        + \ci \omega_{\text{q}} P_{ge} - \gamma_{2,ge} P_{ge}
\\ 
    \dot{P}_{eg}
    &= \frac{\partial}{\partial \alpha}
        \left[
            (- \ci \epsilon 
            + \ci \chi_{\text{qr}} \alpha
            + \ci \Delta_{\text{rd}} \alpha 
            + \kappa \alpha/2) 
            P_{eg}
        \right]
        + \frac{\partial}{\partial \beta}
        \left[
            (\ci \epsilon^{*}  
            - \ci \Delta_{\text{rd}} \beta
            + \kappa \beta/2) 
            P_{eg}
        \right]
\nonumber \\ \label{eq:complex_P_eg}
    & \ \ \ \ \ \ \ \ \ \ \ \ \ \ \ \ \ \ \ \ \ \ \ \ \ \ \ \ \ \ \ \ \ \ \ \ \ \ \ \ \ \ \ \ \ \ \ \ \ \ \ \ \ \ \ \ \ \ \ \
        - \ci \chi_{\text{qr}} \alpha \beta P_{eg}
        - \ci \omega_{\text{q}} P_{eg} - \gamma_{2,ge} P_{eg}
\\ 
    \dot{P}_{gf}
    &= \frac{\partial}{\partial \alpha}
        \left[
            (- \ci \epsilon 
            + \ci \Delta_{\text{rd}} \alpha 
            + \kappa \alpha/2) 
            P_{gf}
        \right]
        + \frac{\partial}{\partial \beta}
        \left[
            (\ci \epsilon^{*}  
            - \ci 2\chi_{\text{qr}} \beta
            - \ci \Delta_{\text{rd}} \beta
            + \kappa \beta/2) 
            P_{gf}
        \right]
\nonumber \\ \label{eq:complex_P_gf}
    & \ \ \ \ \ \ \ \ \ \ \ \ \ \ \ \ \ \ \ \ \ \ \ \ \ \ \ \ \ \ \ \ \ \ \ \ \ \ \ \ \ \ \ \ \ \ \ \ \ \ \ \ \ \ \ \ \ \ \ \
        + \ci 2\chi_{\text{qr}} \alpha \beta P_{gf}
        + \ci (2\omega_{\text{q}} + \alpha_{\text{q}}) P_{gf} - \gamma_{2,gf} P_{gf}
\\ 
    \dot{P}_{fg}
    &= \frac{\partial}{\partial \alpha}
        \left[
            (- \ci \epsilon 
            + \ci 2\chi_{\text{qr}} \alpha 
            + \ci \Delta_{\text{rd}} \alpha 
            + \kappa \alpha/2) 
            P_{fg}
        \right]
        + \frac{\partial}{\partial \beta}
        \left[
            (\ci \epsilon^{*}  
            - \ci \Delta_{\text{rd}} \beta
            + \kappa \beta/2) 
            P_{fg}
        \right]
\nonumber \\ \label{eq:complex_P_fg}
    & \ \ \ \ \ \ \ \ \ \ \ \ \ \ \ \ \ \ \ \ \ \ \ \ \ \ \ \ \ \ \ \ \ \ \ \ \ \ \ \ \ \ \ \ \ \ \ \ \ \ \ \ \ \ \ \ \ \ \ \
        - \ci 2\chi_{\text{qr}} \alpha \beta P_{fg}
        - \ci (2\omega_{\text{q}} + \alpha_{\text{q}}) P_{fg} - \gamma_{2,gf} P_{fg}
\\ 
    \dot{P}_{ef}
    &= \frac{\partial}{\partial \alpha}
        \left[
            (- \ci \epsilon 
            + \ci \chi_{\text{qr}} \alpha 
            + \ci \Delta_{\text{rd}} \alpha 
            + \kappa \alpha/2) 
            P_{ef}
        \right]
        + \frac{\partial}{\partial \beta}
        \left[
            (\ci \epsilon^{*}  
            - \ci 2\chi_{\text{qr}} \beta
            - \ci \Delta_{\text{rd}} \beta
            + \kappa \beta/2) 
            P_{ef}
        \right]
\nonumber \\ \label{eq:complex_P_ef}
    & \ \ \ \ \ \ \ \ \ \ \ \ \ \ \ \ \ \ \ \ \ \ \ \ \ \ \ \ \ \ \ \ \ \ \ \ \ \ \ \ \ \ \ \ \ \ \ \ \ \ \ \ \ \ \ \ \ \ \ \
        + \ci \chi_{\text{qr}} \alpha \beta P_{ef}
        + \ci (\omega_{\text{q}} + \alpha_{\text{q}}) P_{ef} - \gamma_{2,ef} P_{ef}
\\ 
    \dot{P}_{fe}
    &= \frac{\partial}{\partial \alpha}
        \left[
            (- \ci \epsilon 
            + \ci 2\chi_{\text{qr}} \alpha 
            + \ci \Delta_{\text{rd}} \alpha 
            + \kappa \alpha/2) 
            P_{fe}
        \right]
        + \frac{\partial}{\partial \beta}
        \left[
            (\ci \epsilon^{*}  
            - \ci \chi_{\text{qr}} \beta
            - \ci \Delta_{\text{rd}} \beta
            + \kappa \beta/2) 
            P_{fe}
        \right]
\nonumber \\ \label{eq:complex_P_fe}
    & \ \ \ \ \ \ \ \ \ \ \ \ \ \ \ \ \ \ \ \ \ \ \ \ \ \ \ \ \ \ \ \ \ \ \ \ \ \ \ \ \ \ \ \ \ \ \ \ \ \ \ \ \ \ \ \ \ \ \ \
        - \ci \chi_{\text{qr}} \alpha \beta P_{fe}
        - \ci (\omega_{\text{q}} + \alpha_{\text{q}}) P_{fe} - \gamma_{2,ef} P_{fe}
\end{align}

Although looks complicated, the nine coupled equations admit simple trajectories in the complex plane of $\alpha$ and $\beta$. We use the ansatze
\begin{align}
    P_{gg}(\alpha, \beta, t)
    &= \delta^{(2)}(\alpha - \alpha_g(t)) 
        \delta^{(2)}(\beta - \alpha_g^*(t))
\\
    P_{ee}(\alpha, \beta, t)
    &= \delta^{(2)}(\alpha - \alpha_e(t)) 
        \delta^{(2)}(\beta - \alpha_e^*(t))
\\ 
    P_{ff}(\alpha, \beta, t)
    &= \delta^{(2)}(\alpha - \alpha_f(t)) 
        \delta^{(2)}(\beta - \alpha_f^*(t))
\\
    P_{ge}(\alpha, \beta, t)
    &= c_{ge}(t) \delta^{(2)}(\alpha - \alpha_g(t)) 
        \delta^{(2)}(\beta - \alpha_e^*(t))
\\
    P_{eg}(\alpha, \beta, t)
    &= c_{eg}(t) \delta^{(2)}(\alpha - \alpha_e(t)) 
        \delta^{(2)}(\beta - \alpha_g^*(t))
\\ 
    P_{gf}(\alpha, \beta, t)
    &= c_{gf}(t) \delta^{(2)}(\alpha - \alpha_g(t)) 
        \delta^{(2)}(\beta - \alpha_f^*(t))
\\ 
    P_{fg}(\alpha, \beta, t)
    &= c_{fg}(t) \delta^{(2)}(\alpha - \alpha_f(t)) 
        \delta^{(2)}(\beta - \alpha_g^*(t))
\\ 
    P_{ef}(\alpha, \beta, t)
    &= c_{ef}(t) \delta^{(2)}(\alpha - \alpha_e(t)) 
        \delta^{(2)}(\beta - \alpha_f^*(t))
\\
    P_{fe}(\alpha, \beta, t)
    &= c_{fe}(t)\delta^{(2)}(\alpha - \alpha_f(t)) 
        \delta^{(2)}(\beta - \alpha_e^*(t)).
\end{align}
Each diagonal term $P_{aa}$ represents a single coherent state whose amplitudes are specified by the two delta functions. Plug the ansatze into Eq.(\ref{eq:complex_P_gg})-(\ref{eq:complex_P_ff}), we obtain the time evolution of the coherent states 
\begin{align} \label{eq:differential_eqn_alpha_g}
    \dot{\alpha}_g
    &= - \ci (\Delta_{\text{rd}} - \ci \kappa/2) \alpha_g
        + \ci \epsilon
\\ \label{eq:differential_eqn_alpha_e}
    \dot{\alpha}_e
    &=  - \ci (\Delta_{\text{rd}} + \chi_{\text{qr}} - \ci \kappa/2) \alpha_e
        + \ci \epsilon
\\ \label{eq:differential_eqn_alpha_f}
    \dot{\alpha}_f
    &= - \ci (\Delta_{\text{rd}} + 2 \chi_{\text{qr}} - \ci \kappa/2) \alpha_f
        + \ci \epsilon.
\end{align}
Besides the time evolution brought by the coherent states, each non-diagonal term $P_{ab}$ ($a \neq b$) is modulated by an envelope function $c_{ab}$. By substituting the ansatze together with Eq.(\ref{eq:differential_eqn_alpha_g})-(\ref{eq:differential_eqn_alpha_f}) into Eq.(\ref{eq:complex_P_ge})-(\ref{eq:complex_P_fe}), we deduce that
\begin{align}
    \dot{c}_{ge}
    &= \ci(\omega_{\text{q}} + \ci \gamma_{2,ge}) c_{ge} 
        + \ci \chi_{\text{qr}} \alpha_g \alpha_e^* c_{ge}
\\ 
    c_{eg}
    &= c_{ge}^{*}
\\
    \dot{c}_{gf}
    &= \ci(2\omega_{\text{q}} + \alpha_{\text{q}} + \ci \gamma_{2,gf}) c_{gf} 
        + \ci 2\chi_{\text{qr}} \alpha_g \alpha_f^* c_{gf}
\\ 
    c_{fg}
    &= c_{gf}^{*}
\\
    \dot{c}_{ef}
    &= \ci(\omega_{\text{q}} + \alpha_{\text{q}} + \ci \gamma_{2,ef}) c_{ef} 
        + \ci \chi_{\text{qr}} \alpha_e \alpha_f^* c_{ef}
\\ 
    c_{fe}
    &= c_{ef}^{*}
\end{align}

Given the initial conditions, the time evolution of $\alpha_{a}$ and $c_{ab}$ can be solved easily. After integrating the delta functions in the complex plane of $\alpha$ and $\beta$, we arrive at the general solution (in the rotating frame)
\begin{align*}
    \hat{\rho}_{\mathcal{SR}}(t) 
    &= P_g(0) \ket{g} \! \bra{g} \otimes  \ket{\alpha_g(t)} \! \bra{\alpha_g(t)}
    + P_e(0) \ket{e} \! \bra{e} \otimes  \ket{\alpha_e(t)} \! \bra{\alpha_e(t)}
    + P_f(0) \ket{f} \! \bra{f} \otimes  \ket{\alpha_f(t)} \! \bra{\alpha_f(t)}
\nonumber \\
    &\ \ \ \ 
    + \frac{a_{ge}(t)}{\bra{\alpha_{e}(t)}\ket{\alpha_g(t)}} \ket{g} \! \bra{e} \otimes  \ket{\alpha_g(t)} \! \bra{\alpha_e(t)}
    + \frac{a_{eg}(t)}{\bra{\alpha_{g}(t)}\ket{\alpha_e(t)}} \ket{e} \! \bra{g} \otimes  \ket{\alpha_e(t)} \! \bra{\alpha_g(t)}
\nonumber \\
    &\ \ \ \ + \frac{a_{gf}(t)}{\bra{\alpha_{f}(t)}\ket{\alpha_g(t)}} \ket{g} \! \bra{f} \otimes  \ket{\alpha_g(t)} \! \bra{\alpha_f(t)}
    + \frac{a_{fg}(t)}{\bra{\alpha_{g}(t)}\ket{\alpha_f(t)}} \ket{f} \! \bra{g} \otimes  \ket{\alpha_f(t)} \! \bra{\alpha_g(t)}
\nonumber \\
    &\ \ \ \ + \frac{a_{ef}(t)}{\bra{\alpha_{f}(t)}\ket{\alpha_e(t)}} \ket{e} \! \bra{f} \otimes  \ket{\alpha_e(t)} \! \bra{\alpha_f(t)}
    + \frac{a_{fe}(t)}{\bra{\alpha_{e}(t)}\ket{\alpha_f(t)}} \ket{f} \! \bra{e} \otimes  \ket{\alpha_f(t)} \! \bra{\alpha_e(t)}
\end{align*}

Of particular interest is the steady-state amplitudes of the cavity coherent states
\begin{align}
    \alpha_g (+\infty)
    &= \frac{\sqrt{\kappa} \bar{a}_{\text{in}}}{\Delta_{\text{rd}} - \ci \kappa/2}
\\ 
    \alpha_e (+\infty)
    &= \frac{\sqrt{\kappa} \bar{a}_{\text{in}}}{\Delta_{\text{rd}} + \chi_{\text{qr}} - \ci \kappa/2}
\\ 
    \alpha_f (+\infty)
    &= \frac{\sqrt{\kappa} \bar{a}_{\text{in}}}{\Delta_{\text{rd}} + 2\chi_{\text{qr}} - \ci \kappa/2},
\end{align}
which are the kind of result we would expect from the QLE when driven by a classical source.
